# Supplementary material for: PixMIM: Rethinking Pixel Reconstruction in Masked Image Modeling
Source: arXiv:2303.02416 source file (2023-03-24)
Supplement: Supplementary file 1 [file 2x.tex]

\begin{table}[h]
\tablestyle{6pt}{1.02}
\begin{tabular}{y{96}|y{68}}
config & value \\
\shline
optimizer & AdamW\cite{adamw} \\
base learning rate & 8e-5 \\
weight decay & 0.1 \\
optimizer momentum & $\beta_1, \beta_2{=}0.9, 0.999$ \\
layer-wise lr decay \cite{electra,BEiT} & 0.75 \\
batch size & 64 \\
learning rate schedule & cosine decay \\
training epochs & 100/50  \\
drop path \cite{droppath} & 0.1 \\
\end{tabular}
\caption{{End-to-end object detection setting of \ourmethod$_\text{\tt MAE}$ and \ourmethod$_\text{\tt LSMAE}$}}
\label{tab:impl_lsmae_det} \vspace{-.5em}
\end{table}
