# Supplementary material for: PixMIM: Rethinking Pixel Reconstruction in Masked Image Modeling
Source: arXiv:2303.02416 source file (2023-03-24)
Supplement: Supplementary file 2 [file convmae_pretrain.tex]

\begin{table}[h]
\tablestyle{6pt}{1.02}
\scriptsize
\begin{tabular}{y{96}|y{68}}
config & value \\
\shline
optimizer & AdamW \cite{adamw} \\
base learning rate & 1.5e-4 \\
weight decay & 0.05 \\
optimizer momentum & $\beta_1, \beta_2{=}0.9, 0.95$ \cite{pixel} \\
batch size & 4096 \\
learning rate schedule & cosine decay \cite{cosine} \\
warmup epochs \cite{warmup} & 40 \\
augmentation & SimpleResizedCrop \\
\end{tabular}
\vspace{-.5em}
\caption{\textbf{Pre-training setting for ConvMAE+}}
\label{tab:impl_mae_pretrain} \vspace{-.5em}
\end{table}
